# Supplementary material for: UAP-BEV: Uncertainty Aware Planning using Bird's Eye View generated from Surround Monocular Images
Source: arXiv:2306.04939 source file (2023-06-08)
Supplement: Supplementary file 1 [file 09Appendix.tex]

\section{Appendix}

\subsection{Spatio Temporal BEV Generation}
\label{sec:bev_gen}

\Madhav{Is this ditto LSS or STP3 or is there any difference. If it is ditto STP3 do we need this amount of real estate, if it is different in a small way better to say what that is}
% Okay sir i will shorten this part

Motivated by \cite{stp3}, our architecture reasons about spatio-temporal semantic BEV from surround monocular images, taking in camera inputs from past \textit{t} timestamps. 
At the current time instant $t$, we extract features from RGB images $I$ = \{I$_t^1$,I$_t^2$,\dots,I$_t^N$\}, for $i=\{1...N\}$,where N=number of cameras, and $I_t^i\in \mathbb{R}^{H \times W \times 3}$ ($W$ and $H$ are width and height of each image). Each image, $I_t^i$, is passed  through a backbone network $E$ (we use Efficient-net-B0 \cite{efficientnet}) and downsampled by a factor of $16$ to generate a feature embedding $^{\text{context}}\varepsilon_t^i$ = $E(I_t^i) \in \mathbb{R}^{C \times H' \times W'}$ where $\displaystyle{H'=\frac{H}{16}}$ and $\displaystyle{W'=\frac{W}{16}}$ and $C$ = number of image features. Metric depth information is incorporated by reasoning about a discrete probability distribution $d\in[D_{\text{min}},D_{\text{max}}]$ for each pixel (to a resolution of $\Delta d$) in the down sampled image.
Let the depth embedding be denoted by  $^{\text{depth}}\varepsilon_t^i \in \mathbb{R}^{D \times H' \times W'}$ where $\displaystyle{D=\frac{D_{\text{max}}-D_{\text{min}}}{\Delta d}}$. 
For each pixel $(i,j) \in$ $H' \times W'$, the network learns a context vector $c_{ij} \in \mathbb{R}^{C} $ and a discrete depth distribution $d_{ij} \in \mathbb{R}^{D}$. Using outer product $\gamma_t^i=^{\text{context}}\varepsilon_t^i\otimes^{\text{depth}}\varepsilon_t^j\in \mathbb{R}^{C \times D \times H' \times W'}$, the camera features are then modulated by the discrete depth probabilities to form an approximation for self-attention for context features. \\
After that, we use camera parameters (intrinsics and extrinsics) to transform the above camera features $\left\{\gamma _1,\gamma_2,\dots,\gamma_N\right\}$ to the global 3D coordinate with the origin at the center of ego-vehicle at time \textit{t}. Post this, the BEV feature maps $b_i \in \mathbb{R}^{C \times H' \times W'} $ are obtained after sum pooling $\left\{\gamma _i\right\}$ along the vertical dimensions.
After achieving spatial fusion, the BEV feature maps are passed a temporal fusion network comprising of 3D convolutions. The temporally fused features $\left\{x _1,x_2,\dots,x_t\right\}$ are then passed through a GRU to predict future states $\left\{x _{t+1},x_{t+2},\dots,x_{t+h}\right\}$. All the features are then passed through a decoder $D$ to generate BEV representation of the scene.

\begin{table*}[!ht]
\centering
\caption{\scriptsize{List of Inequality Constraints Used in the projection optimization}}
\small
\begin{tabular}{|c|c|c|c|c|c|}
\hline
Constraint Type & Expression & Parameters   \\ \hline
\SelfNote{This row is needed?} Collision Avoidance  & $-\frac{(x(t)-x_{o, i}(t))^2}{a^2}-\frac{(y(t)-y_{o, i}(t))^2}{b^2}+1\leq 0$ & \makecell{$\frac{a}{2}, \frac{b}{2}$: axis of the circumscribing ellipse \\ of vehicle footprint. \\ $x_{o,i}(t), y_{o, i}(t)$: trajectory of neighboring vehicles} \\ \hline
Velocity bounds & $\sqrt{\dot{x}(t)^2+\dot{y}(t)^2}\leq v_{max}$ & $v_{max}$: maximum velocity of the ego-vehicle   \\ \hline
Acceleration bounds & $\sqrt{\ddot{x}(t)^2+\ddot{y}(t)^2}\leq a_{max}$ & $a_{max}$: maximum acceleration of the ego-vehicle  \\ \hline
Lane boundary & $l_{lb}\leq y(t)\leq l_{ub}$ & \makecell{$y_{lb}, y_{ub}$: Lane bounds.} \\ \hline
\end{tabular}
\normalsize
\label{ineq_list}
\vspace{-0.6cm}
\end{table*}
\normalsize

\subsection{Reformulating Constraints:} 
\SelfNote{Do we add Obstacle Avoidance Constraints?}

\noindent Table \ref{ineq_list} presents the list of all the constraints included in our projection optimizer. The collision avoidance constraints presented there can be re-written in the following form:

\small
\begin{align}
    \textbf{f}_{o, i} = \left \{ \begin{array}{lcr}
x(t) -x_{o, i}(t)-d_{o, i}(t)\cos\alpha_{o, i}(t) \\
y(t) -y_{o, i}(t)-d_{o, i}(t)\sin\alpha_{o, i}(t) \\ 
\end{array} \right \} d_{o, i}(t)\geq 1
\label{sphere_proposed}
\end{align}
\normalsize
\vspace{-0.1cm}
\noindent where $\alpha_{o, i}(t)$ represents the angle that the line-of-sight vector between the ego-vehicle and its $i^{th}$ neighbor makes with the $X$ axis. Similarly, the variable $d_{o, i}(t)$ represents the ratio of the length of this vector with the minimum distance separation required for collision avoidance. Following a similar approach, we can rephrase the velocity and acceleration bounds from Table \ref{ineq_list} as:

\vspace{-0.3cm}

\small
\begin{align}
    \textbf{f}_{v} = \left \{ \begin{array}{lcr}
\dot{x}(t) -d_{v}(t)\cos\alpha_{v}(t) \\
\dot{y}(t) -d_{v}(t)\sin\alpha_{v}(t)\\ 
\end{array} \right \}, v_{min}\leq d_{v}(t)\leq v_{max}
\label{vel_bound_proposed}
\end{align}
\normalsize

\vspace{-0.5cm}
\small
\begin{align}
    \textbf{f}_{a} = \left \{ \begin{array}{lcr}
\ddot{x}(t) -d_{a}(t)\cos\alpha_{a}(t) \\
\ddot{y}(t) -d_{a}(t)\sin\alpha_{a}(t)\\ 
\end{array} \right \}, 0\leq d_{a}(t)\leq a_{max}
\label{acc_bound_proposed}
\end{align}
\normalsize

The variables $\alpha_{o, i}(t)$, $\alpha_{o, i}(t)$, $\alpha_{a, i}(t)$, $d_{o, i}(t)$, $d_{v, i}(t)$, and $d_{a, i}(t)$  are additional variables that will be obtained by our batch projection optimizer along with $\overline{\boldsymbol{\xi}}_j^*$.

\subsubsection{Reformulated Problem} Using the developments in the previous section and the trajectory parametrization presented in \eqref{param}, we can now replace the projection optimization \eqref{projection_cost}-\eqref{projection_const} with the following. Note that \eqref{lane_reform} is the matrix representation of the lane boundary constraints presented in Table \ref{ineq_list}.

\small
\begin{subequations}
\begin{align}
    \overline{\boldsymbol{\xi}}_j^{*} = \arg\min_{\overline{\boldsymbol{\xi}}^*_j}\frac{1}{2}\Vert \overline{\boldsymbol{\xi}}^*_j-{\boldsymbol{\xi}}_j^*\Vert_2^2\label{cost_reform}  \\
    \textbf{A} \overline{\boldsymbol{\xi}}^*_j= \textbf{b}(\textbf{p}_j) \label{eq_reform} \\
    \widetilde{\textbf{F}} \hspace{0.05cm} \overline{\boldsymbol{\xi}}^*_j = \widetilde{\textbf{e}}(\boldsymbol{\alpha}_j, \textbf{d}_j) \label{nonconvex_reform}  \\
    \textbf{d}_{min} \leq \textbf{d}_j\leq \textbf{d}_{max} \label{d_reform_1}\\
     \textbf{G}\overline{\boldsymbol{\xi}}^*_j \leq \textbf{y}_{lane} \label{lane_reform}
\end{align}
\end{subequations}
\normalsize

\small
\begin{align}
    \widetilde{\textbf{F}} = \begin{bmatrix}
    \begin{bmatrix}
    \textbf{F}_{o}\\
    \dot{\textbf{W}}\\
    \ddot{\textbf{W}}
    \end{bmatrix} & \textbf{0}\\
    \textbf{0} & \begin{bmatrix}
    \textbf{F}_{o}\\
    \dot{\textbf{W}}\\
    \ddot{\textbf{W}}
    \end{bmatrix} 
    \end{bmatrix}, \widetilde{\textbf{e}} = \begin{bmatrix}
    \textbf{x}_o+a \textbf{d}_{o, j}\cos\boldsymbol{\alpha}_{o, j}\\
     \textbf{d}_{v, j}\cos\boldsymbol{\alpha}_{v, j}\\
  \textbf{d}_{a, j}\cos\boldsymbol{\alpha}_{a, j}\\
 \textbf{y}_o+a \textbf{d}_{o, j}\sin\boldsymbol{\alpha}_{o, j}\\
     \textbf{d}_{v, j}\sin\boldsymbol{\alpha}_{v, j}\\
  \textbf{d}_{a, j}\sin\boldsymbol{\alpha}_{a, j}\\
    \end{bmatrix},
\end{align}
\normalsize
\begin{align}
    \textbf{G} = \begin{bmatrix}
        \textbf{W}\\
        -\textbf{W}
    \end{bmatrix}, \textbf{y}_{lane} = \begin{bmatrix}
        y_{ub} & \dots y_{ub} & y_{lb} \dots y_{lb}
    \end{bmatrix}^T
\end{align}

\small
\begin{align*}
    \boldsymbol{\alpha}_j = (\boldsymbol{\alpha}_{o, j}, \boldsymbol{\alpha}_{a,j}, \boldsymbol{\alpha}_{v,j}), \qquad \textbf{d}_j =  (\textbf{d}_{o, j}, \textbf{d}_{v, j}, \textbf{d}_{a, j})
\end{align*}
\normalsize

\noindent Constraints \eqref{nonconvex_reform}-\eqref{lane_reform} acts as substitutes for $\textbf{g}(\boldsymbol{\xi}_j)\leq 0 $ in the projection optimization \eqref{projection_cost}-\ref{projection_const}. 
% Please also note the addition of subscript $j$ indicating that the \eqref{cost_reform}-\eqref{lane_reform} is defined for the $j^{th}$ sample of ${\boldsymbol{\xi}}_j$

The matrix $\textbf{F}_o$ is obtained by stacking the matrix $\textbf{W}$ from (\ref{param}) as many times as the number of neighboring vehicles considered for collision avoidance at a given planning cycle. The vector $\textbf{x}_o, \textbf{y}_o$ is formed by appropriately stacking $x_{o, i}(t), y_{o, i}(t)$ at different time instants and for all the neighbors. Similar construction is followed to obtain $\boldsymbol{\alpha}_{o}, \boldsymbol{\alpha}_{v}, \boldsymbol{\alpha}_{a}, \textbf{d}_{o}, \boldsymbol{d}_{v} \boldsymbol{d}_{a}$. The vector $\textbf{y}_{lane}$ is formed by stacking the upper and lower lane bounds after repeating them $m$ times (planning horizon). Similarly,  vectors $d_{min}, d_{max}$ are formed by stacking the lower and upper bounds for $d_{o, i}(t), d_a(t), d_v(t)$. Note that the upper bound for $d_{o, i}(t)$ can be simply some large number (recall \eqref{sphere_proposed}). Moreover, these bounds are the same across all batches.

\subsubsection{Solution Process} We relax the non-convex equality \eqref{nonconvex_reform} and affine inequality constraints as $l_2$ penalties and augment them into the projection cost \eqref{cost_reform}.

\small
\begin{dmath}
    \mathcal{L} = \frac{1}{2}\left\Vert \overline{\boldsymbol{\xi}}^*_j-\boldsymbol{\xi}^*_j\right\Vert_2^2- \boldsymbol{\lambda}_{j}^T, \overline{\boldsymbol{\xi}}^*_j+\frac{\rho}{2} \left \Vert \widetilde{\textbf{F}} \overline{\boldsymbol{\xi}}^*_j-\widetilde{\textbf{e}}\right \Vert_2^2+  \frac{\rho}{2}\left \Vert \mathbf{G} \boldsymbol{\xi}_{j} - \textbf{y}_{lane} + \mathbf{s}_j \right \Vert^2 = \frac{1}{2}\left\Vert \overline{\boldsymbol{\xi}}^*_j-\boldsymbol{\xi}^*_j\right\Vert_2^2-\boldsymbol{\lambda}_{j}^T, \overline{\boldsymbol{\xi}}^*_j+\frac{\rho}{2} \left \Vert \textbf{F} \overline{\boldsymbol{\xi}}^*_j-\textbf{e}\right \Vert_2^2
    \label{aug_lag}
\end{dmath}
\normalsize
\begin{align}
    \textbf{F} = \begin{bmatrix}
        \widetilde{\textbf{F}}\\
        \textbf{G}
    \end{bmatrix}, \textbf{e} = \begin{bmatrix}
        \widetilde{\textbf{e}}\\
        \textbf{y}_{lane}-\textbf{s}_j
    \end{bmatrix}
\end{align}

\noindent Note, introducing the Lagrange multiplier $\boldsymbol{\lambda}$ that drives the residual of the second and third quadratic penalties to zero \cite{split_bregman}.

We minimize \eqref{aug_lag} subject to \eqref{eq_reform} through Alternating Minimization (AM), which reduces to the following steps.

\small
\begin{subequations}
    \begin{align}
        {^{k+1}\boldsymbol{\alpha}_j} = \arg\min_{\boldsymbol{\alpha}_j} \mathcal{L}({^k}\overline{\boldsymbol{\xi}}_j^*, {^k}\textbf{d}_j, \boldsymbol{\alpha}_j {^k}\boldsymbol{\lambda}_j, {^k}\textbf{s}_j ) \label{am_alpha}\\
        {^{k+1}\textbf{d}_j} = \arg\min_{\textbf{d}_j} \mathcal{L}({^k}\overline{\boldsymbol{\xi}}_j^*, \textbf{d}_j, {^{k+1}}\boldsymbol{\alpha}_j, {^k}\boldsymbol{\lambda}_j, {^k}\textbf{s}_j) \label{am_d} \\ 
        {^{k+1}}\mathbf{s} =\text{max}\left(0, -\mathbf{G} {^{k}}\overline{\boldsymbol{\xi}}_{j}^* - \textbf{y}_{lane}\right) \label{am_s} \\
        {^{k+1}}\boldsymbol{\lambda}_j = \overbrace{{^{k}}\boldsymbol{\lambda}_j+\rho\textbf{F}^T (\textbf{F}\hspace{0.05cm} {^k}\boldsymbol{\xi}_j^*-{^{k}}\textbf{e}_j  )}^{\textbf{h}_1} \label{am_lambda} \\
        {^{k+1}}\textbf{e}_j = \overbrace{\begin{bmatrix}
        \widetilde{\textbf{e}} ({^{k+1}} \boldsymbol{\alpha}_j, {^{k+1}}\textbf{d}_j ) \label{am_e} \\
        \textbf{y}_{lane}-{^{k+1}}\textbf{s}_j
    \end{bmatrix}}^{\textbf{h}_2}\\
        {^{k+1}}\overline{\boldsymbol{\xi}}_j^* = \arg\min_{\overline{\boldsymbol{\xi}}_j^*}\mathcal{L}(\overline{\boldsymbol{\xi}}_j^*, {^{k+1}}\boldsymbol{\lambda}_j, {^{k+1}}\textbf{e}_j ) \label{am_xi}
    \end{align}
\end{subequations}
\normalsize

As can be seen, we optimize over only one group of variables at each AM step  while others are held fixed at values obtained at the previous updates. Steps \eqref{am_lambda}-\eqref{am_e} provides the function $\textbf{h}$ presented in \eqref{fixed_point_1}. That is, $\textbf{h} = (\textbf{h}_1, \textbf{h}_2)$. Step \eqref{am_xi} represents \eqref{fixed_point_2}.
